# Supplementary material for: Establishing tool support for a concept DSL
Source: arXiv:2503.05849 source file (2025-03-07)
Supplement: Supplementary file 2 [file semantics.tex]

{
\mathlig{->}{\rightarrow}
\mathlig{|-}{\vdash}
\mathlig{=>}{\Rightarrow}
\mathligson

\renewcommand{\inference}[3][]{%
  \begin{array}[b]{@{}c@{}l@{}}
    \smash{\raisebox{-.5\normalbaselineskip}{\footnotesize #1}} & 
      \begin{array}[b]{l}
        #2
      \end{array} \\
      \cline{2-2}
    & \begin{array}[t]{l}
        #3
      \end{array}
  \end{array}
}

\section{Test Semantics}

\inference[]{
x = 0
}{x 0 }
}
